# Supplementary material for: Non-monotonic hydration dependence of ionic transport in atomically-thin MnO2 sheets
Source: arXiv:2601.14836 source file (2026-09-15)
Supplement: Supplementary file 1 [file Supplementary_Information.pdf]

# Supplementary Information: Ionic transport in spontaneously ion-intercalated van der Waals layered structures

Ata Utku Özkan,[*,†,¶] T. Serkan Kasırga,[*,‡,¶] and Aykut Erbaş[*,†,¶]

†Institute of Materials Science and Nanotechnology, Bilkent University, Ankara 06800, Turkiye

‡Department of Physics, Middle East Technical University, Ankara 06800, Turkiye

¶Bilkent National Nanotechnology Research Center - UNAM, Ankara 06800, Turkiye

E-mail: utku.ozkan@bilkent.edu.tr; kasirga@unam.bilkent.edu.tr; aykut.erbas@unam.bilkent.edu.tr

**MnO parameters:**

| Element | Charge(e) | $D_0$ (kcal/mol) | $R_0$ (Å) |
|---|---|---|---|
| Mn | 1.85 | 9.0298e-07 | 5.5070 |
| O | -1.05 | 0.1554 | 3.5532 |
| Na | 1 | 0.1301 | 2.6378 |

**Water parameters:**

| Element | Charge(e) | $D_0$ (kcal/mol) | $R_0$ (Å) |
|---|---|---|---|
| O | -0.8476 | 0.1554 | 3.5532 |
| H | 0.4238 | - | - |

| Bond type | $k$ (kcal/mol Å$^2$) | $r_0$ (Å) |
|---|---|---|
| O-H | 554.1349 | 1.0000 |

| Angle | $k$ (kcal/mol rad$^2$) | $\theta_0$ (deg) |
|---|---|---|
| H-O-H | 45.7696 | 109.47 |

**TABLE S1**: CLAYFF force-field parameters.[1-3]

| $E_x$ | τ (ns) | $\langle v_x \rangle$ (Å/ns) | $c_1$ | $c_2$ | $\langle v_l \rangle$ (Å/ns) | b |
|---|---|---|---|---|---|---|
| 0.010 | 13.2650 | 0.0055 | 0.6775 | 0.2868 | 0.0062 | 0.9086 |
| 0.015 | 14.1710 | 0.0112 | 2.0343 | 0.6951 | 0.0138 | 2.5089 |
| 0.020 | 16.3553 | 0.0225 | 3.1662 | 1.3233 | 0.0278 | 4.0323 |
| 0.025 | 15.5962 | 0.0312 | 8.4501 | 1.3891 | 0.0391 | 8.6612 |

**TABLE S2**:Displacement curve fit parameters. The equation used to fit displacement curves for $1H_2O \cdot Na$ is given by $\Delta x = c_1(1 - exp(- t/\tau)) + \langle v_t \rangle t + c_2$, where $c_1$ and $c_2$ are fitting constants associated with the initial response and offset, τ is the relaxation timescale, above which a linear increase in the displacement data is observed and $\langle v_t \rangle$ is the steady state ion velocity. As a consistency check, we also fit only the steady state (50–100 ns) with $\Delta x = \langle v_t \rangle t + b$ and report those parameters.

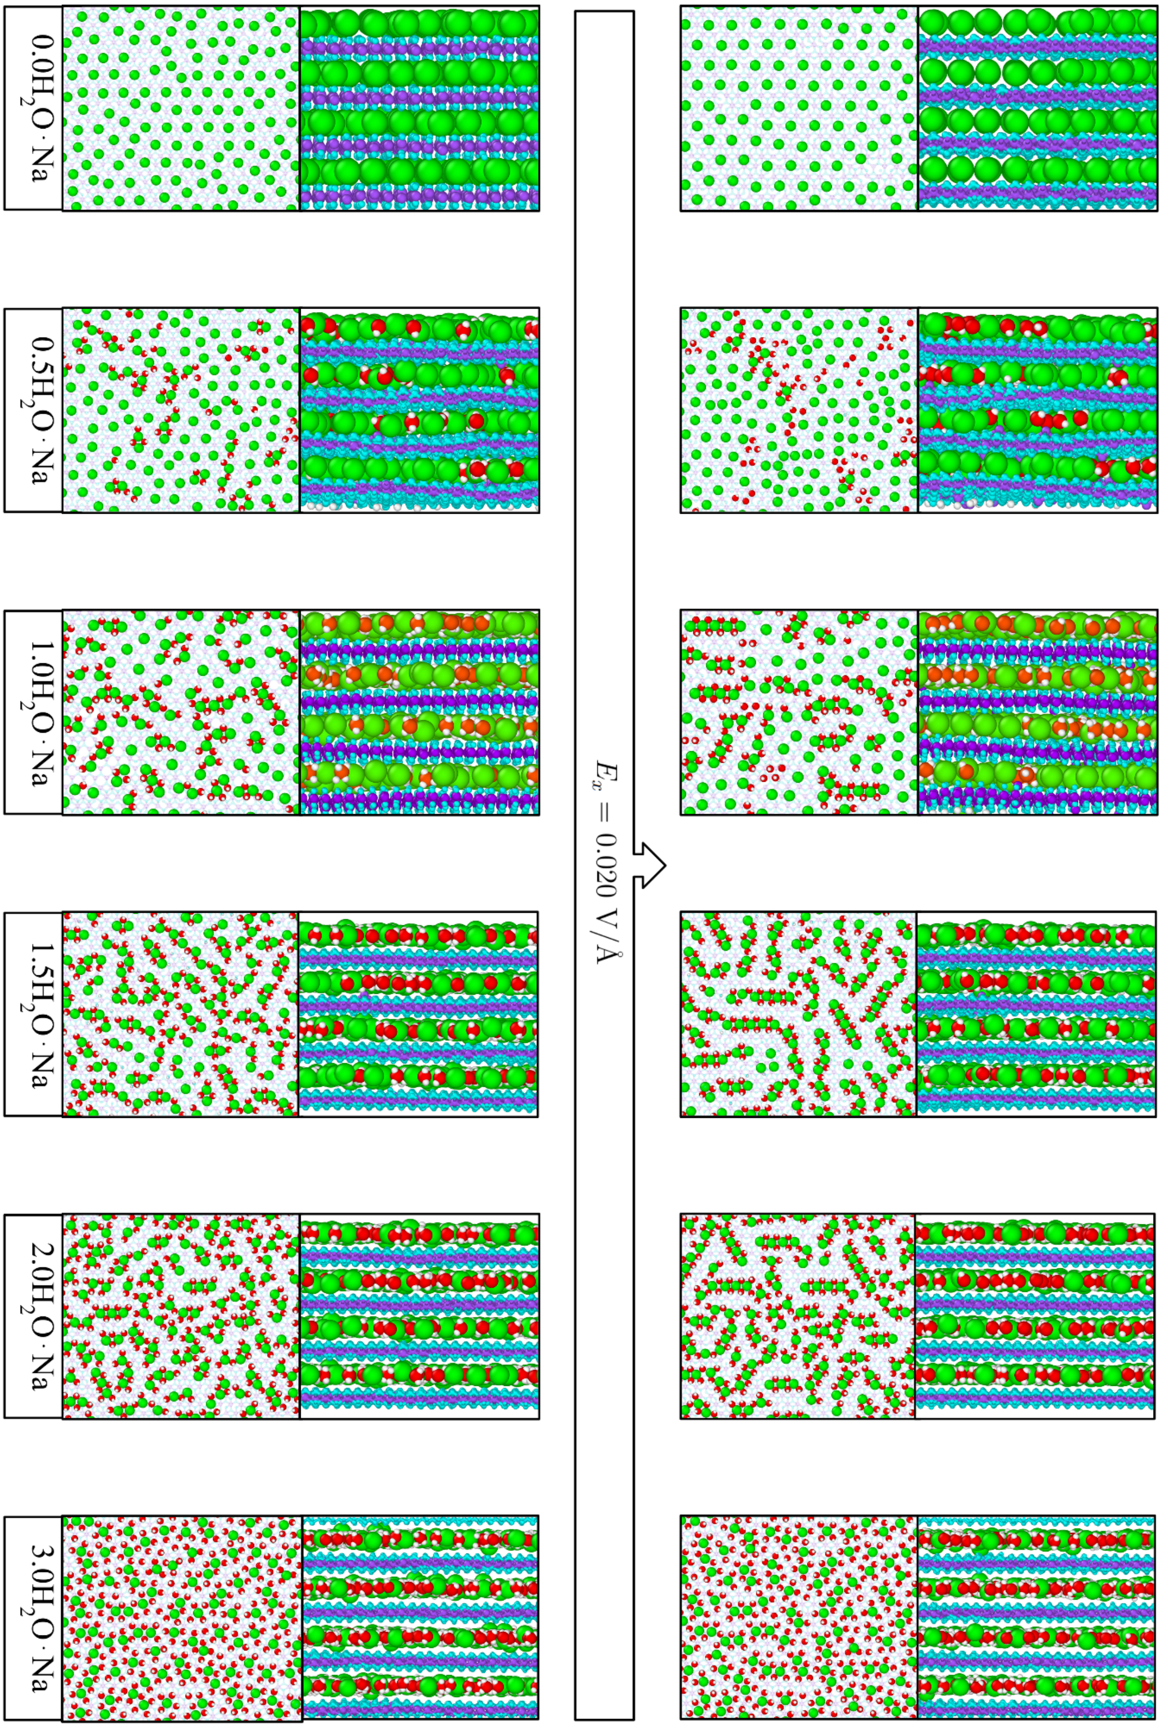


**FIGURE S1**: Interlayer conformations of systems in different water concentrations at equilibrium and after 50 ns under the applied field of $E_x = 0.020$ V/Å.

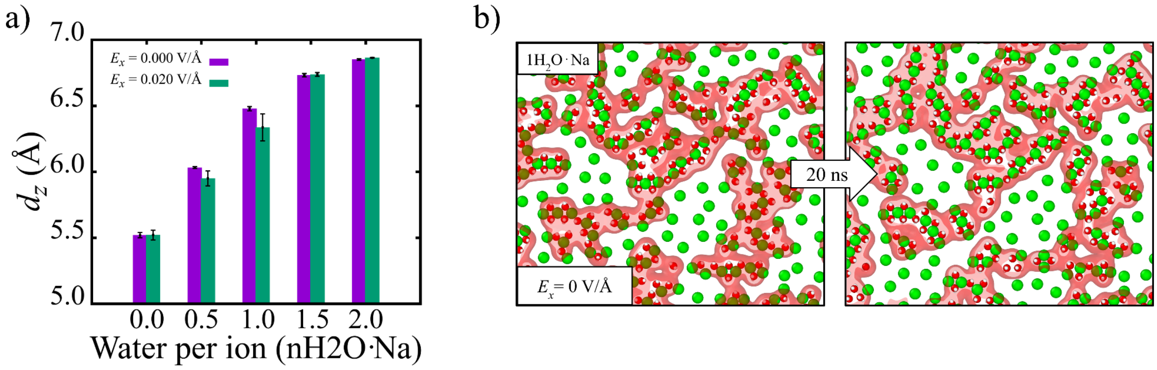


**FIGURE S2:** (a) Interlayer spacing before and after application of an external electric field for different water concentrations. (b) Non-spontaneously rehomogenizing system exhibiting a non-uniform initial water distribution where water molecules are initially distributed non-uniformly and equilibrated in the absence of an external electric field for 20 ns. Water molecules are enclosed by a surface mesh to improve visual clarity.

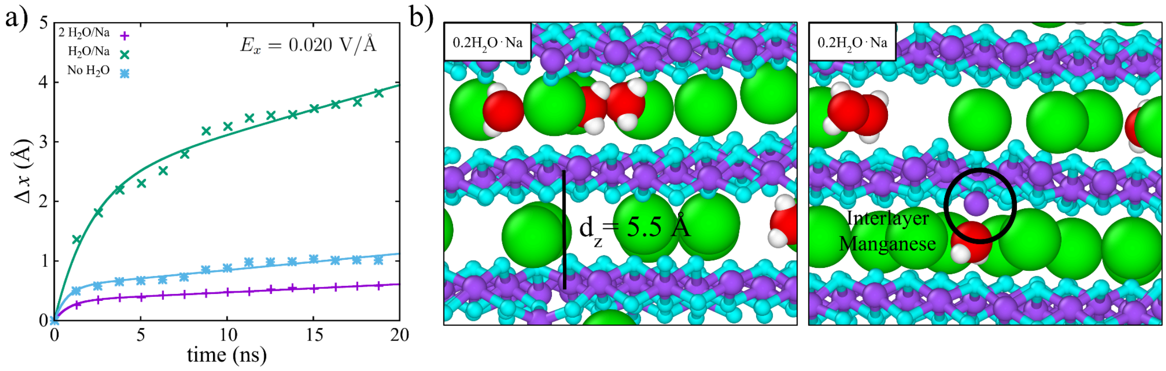


**FIGURE S3:** (a) Displacement trajectories for high- and low-hydration systems, along with (b) low-hydration snapshots illustrating local interlayer collapse and manganese migration into the interlayer region.

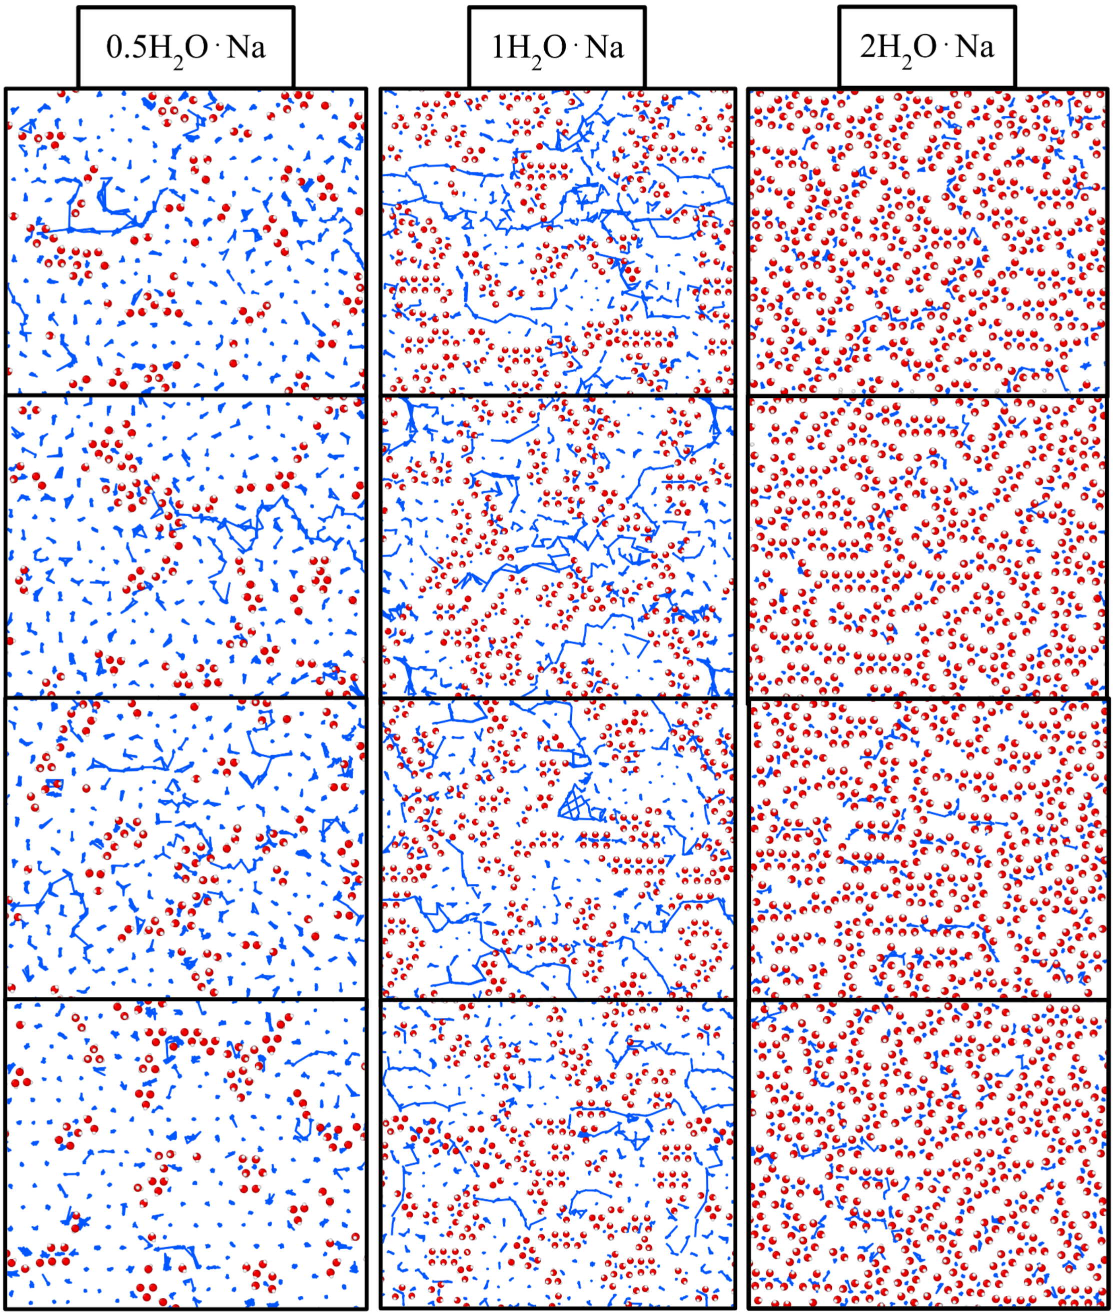


**FIGURE S4**: 50 ns displacement trajectory of sodium ions under different water concentrations with $E_x = 0.020$ V/Å. These trajectories are drawn from the second half of the simulation (50-100 ns), thus do not show the initial redistribution of ions. Blue lines indicate ion movements. Ions are not shown for clarity.

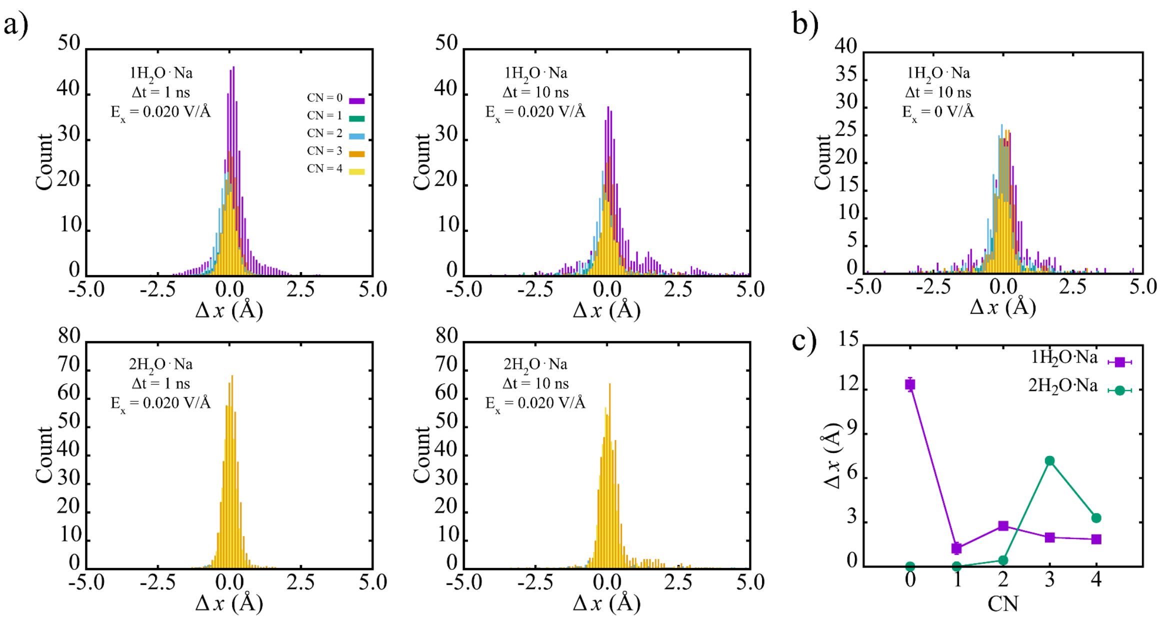


**FIGURE S5**: (a) Displacement histograms of 1 and $2H_2O \cdot Na$ systems binned with different time windows. Ions with the same coordination number (CN) are selected at time t, and their displacements are evaluated relative to the configuration at t+Δt, without imposing conservation of the coordination number between the two frames. Then the displacement values are binned for each CN and averaged over the total number of timeframes. (b) Displacement histograms of the $1H_2O \cdot Na$ system without an applied electric field. (c) Coordination number versus average ionic displacement in 50 ns simulations under an applied field of $E_x = 0.020$ V/Å.

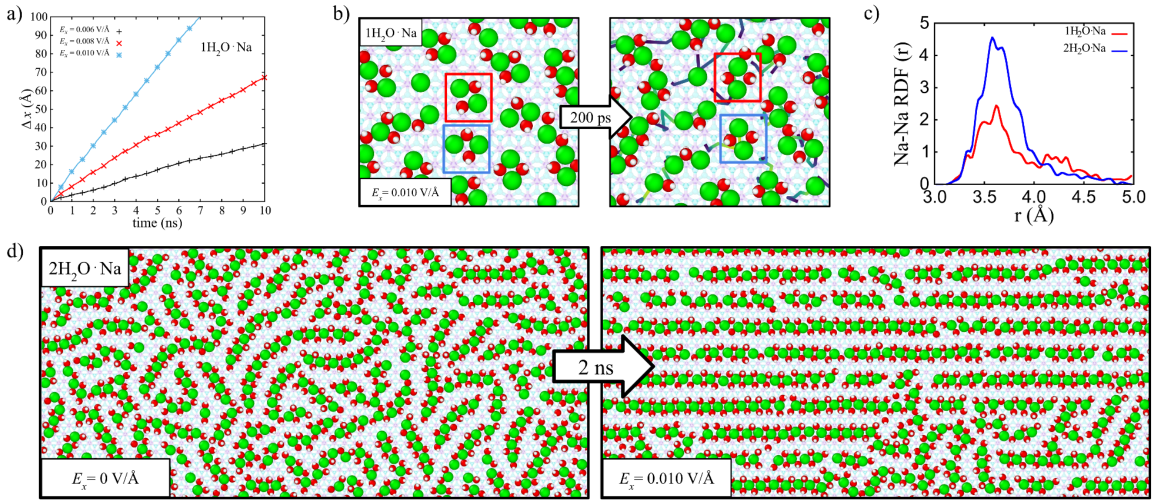


**FIGURE S6**: (a) Displacement trajectories for rigid layer $1H_2O \cdot Na$ systems under various electric fields. (b) Snapshots illustrating the ionic hopping mechanism in rigid-layer $1H_2O \cdot Na$ systems, showing ion migration between neighboring octahedral sites. (c) Sodium-Sodium (Na-Na) radial distribution functions of 1 and $2H_2O \cdot Na$ systems without an applied electric field. (d) Snapshots (2x1x1 system) of organization of filamentous clusters along field direction in $2H_2O \cdot Na$ rigid layer system.

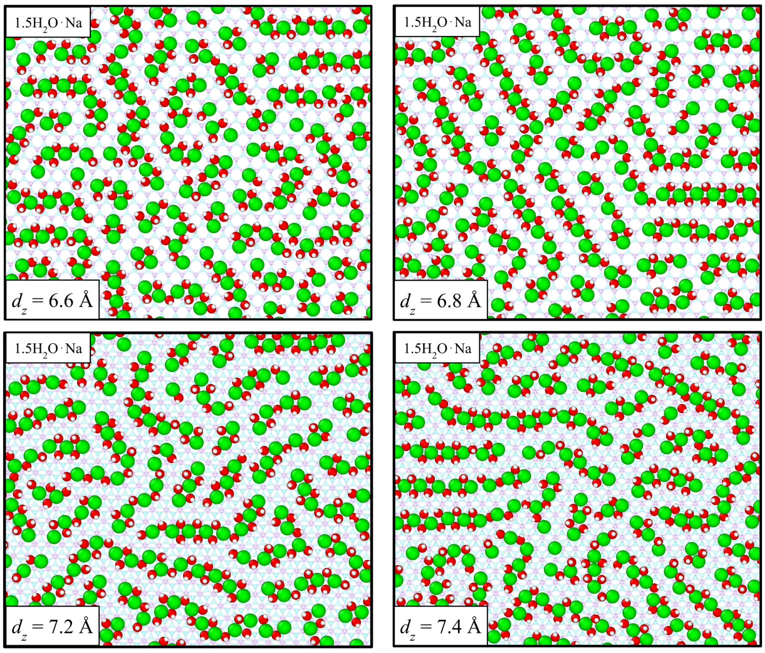


**FIGURE S7**: Snapshots of rigid layer $1.5H_2O \cdot Na$ systems equilibrated without an applied electric field in various interlayer distances demonstrating different sizes of clusters.

References

[1] Cygan, R. T.; Greathouse, J. A.; Kalinichev, A. G. Advances in Clayff Molecular Simulation of Layered and Nanoporous Materials and Their Aqueous Interfaces. The Journal of Physical Chemistry C 2021, 125, 17573–17589

[2] Newton, A. G.; Kwon, K. D. Classical mechanical simulations of layer- and tunnel structured manganese oxide minerals. Geochimica et Cosmochimica Acta 2020, 291, 92–109, Multiscale Simulation in Geochemistry.

[3] Newton, A. G.; Kwon, K. D. Molecular simulations of hydrated phyllomanganates. Geochimica et Cosmochimica Acta 2018, 235, 208–223.
